# Supplementary material for: Predicting vs. Acting: A Trade-off Between World Modeling & Agent Modeling
Source: arXiv:2407.02446 source file (2024-07-02)
Supplement: Supplementary file 1 [file fig-sankey-appendix-5.tex]

\begin{figure}[b!h]
\centering \footnotesize

\begin {minipage}{\textwidth} \centering
\includegraphics[width=1\linewidth]{img/sankey_appendix_rlhf_70b_ex_5}
 \textbf{Llama 70B RLHF, Nucleus Sampling, $p$=0.9}
\end{minipage}
\begin{minipage}{\textwidth} \centering
\includegraphics[width=1\linewidth]{img/sankey_appendix_base_70b_ex_5}
 \textbf{Llama 70B Base, Nucleus Sampling, $p$=0.7}
\end{minipage}
\begin {minipage}{\textwidth} \centering
\includegraphics[width=1\linewidth]{img/sankey_appendix_rlhf_7b_ex_5}
 \textbf{Llama 7B RLHF, Nucleus Sampling, $p$=0.9}
\end{minipage}
\begin{minipage}{\textwidth} \centering
\includegraphics[width=1\linewidth]{img/sankey_appendix_base_7b_ex_5}
 \textbf{Llama 7B Base, Nucleus Sampling, $p$=0.7}
\end{minipage}

\caption{
% \textbf{}
% A Sankey diagram of 100 RLHF model generations for one prompt. Sequences share multiple lengthy anchor spans which appear verbatim in the same order, forming a skeleton for nearly all generations. 
(\S\ref{sec:anchor_spans}) Further examples of Sankey diagrams, as in Figure~\ref{fig:sankey}. Each Sankey diagram visualizes 100 responses (nucleus sampling, p = 0.9 for RLHF and p = 0.7 for Base) to the prompt ``''

}
\label{fig:sankey}
\end{figure}
